# Supplementary material for: Deep Photo Cropper and Enhancer
Source: arXiv:2008.00634 source file (2020-08-03)
Supplement: Supplementary file 1 [file SuppMat.tex]

% % Template for ICIP-2018 paper; to be used with:
% %          spconf.sty  - ICASSP/ICIP LaTeX style file, and
% %          IEEEbib.bst - IEEE bibliography style file.
% % --------------------------------------------------------------------------
% \documentclass{article}
% \usepackage{spconf,amsmath,graphicx}

% \usepackage{color}
% % Example definitions.
% % --------------------
% \def\x{{\mathbf x}}
% \def\L{{\cal L}}

% % Title.
% % ------
% \title{Deep Photo Cropper and Enhancer \\
% Supplementary Materials}
% %
% % Single address.
% % ---------------
% \name{Aaron Ott$^{\ddag}$$^{\star}$   \thanks{$\star$ First and second authors contributed equally.}\qquad Amir Mazaheri$^{\dagger}$$^{\star}$  \qquad Niels D. Lobo$^{\dagger}$ \qquad Mubarak Shah$^{\dagger}$}
  
% \address{$^{\dagger}$ \small Center for Research in Computer Vision (CRCV)-University of Central Florida ~~~
%       $^{\ddag}$ North Carolina State University}

% % \twoauthors
% % {Aaron Ott\thanks{Aaron Ott contributed to this work while he was an NSF REU
% % student at UCF thanks to the support of NSF CNS \#1461121.}}
% % {\small North Carolina State University\\
% % \small apott@ncsu.edu}
% % {Amir Mazaheri, Niels D. Lobo, and Mubarak Shah}{\small Center For Research in Computer Vision (CRCV),
% % University of Central Florida \\
% % \small amirmazaheri@knights.ucf.edu, \{niels, shah\} @cs.ucf.edu}
% %
% % For example:
% % ------------
% %\address{School\\
% %	Department\\
% %	Address}
% %
% % Two addresses (uncomment and modify for two-address case).
% % ----------------------------------------------------------
% %\twoauthors
% %  {A. Author-one, B. Author-two\sthanks{Thanks to XYZ agency for funding.}}
% %	{School A-B\\
% %	Department A-B\\
% %	Address A-B}
% %  {C. Author-three, D. Author-four\sthanks{The fourth author performed the work
% %	while at ...}}
% %	{School C-D\\
% %	Department C-D\\
% %	Address C-D}
% %
% \newcommand{\MS}[1]{{\color{blue}  #1}}
% \begin{document}
% %\ninept
% %
% \maketitle
% %
% % \MS {put the names in one line and put the affiliations on the second line using some kind of indicator like 1 and 2, as other papers do, to save space}
% \section{Supplementary Materials}
% In the main manuscript, we described the new problem of Deep Photo Cropper and Enhancement(DCE) in which the task is to automatically recovering an embedded image within a photo. We show that deep neural networks have the potential to automatically find a transformation which can be applied on a photo and crop the embedded image out of the given photo. Finally, we leverage an enhancer neural network which is an image to CNNs based network. The enhancer increases the quality of the output image since the embedded image might be a small portion of the given photo, have distortions.

% In this supplementary materials document, we provide some details about the proposed network and some more examples of the network output (in addition to the main manuscript) to provide more proofs of the potentials of the proposed network.

% We will publish the dataset, codes for training and testing, and the scripts for generating synthetic data upon the publication of the paper.

% \subsection{Experimental Setup Supplementary Details}
% We train the proposed network with Adam Optimizer~\cite{kingma2014adam} and initial learning rate of $0.0002$. We use \textit{Keras 2.0}\footnote{https://keras.io/} framework to implement, train and test our proposed network. Also, we use Nvidia's Tesla V100 \footnote{https://www.nvidia.com/en-us/data-center/tesla-v100/} GPUs with 16 GB graphical memory to run our experiments. In most of our experiments, the loss value converges after 3-4 hours. We simply use the loss value on training set as our stopping criterion.

% Our proposed model with a single cropper and enhancer has totally ``27,352,833'' parameters in which ``7,325,169'' of them are trainable (we use pre-trained weights of VGG19~\cite{simonyan2014very} and do not change them through the training). Majority of the trainable parameters of the proposed network (``5,807,598'' of the trainable parameters) are for the cropper sub-network.

% \subsection{Qualitative Results} \label{seq:QualResults}
% In Figure~\ref{fig:SDQualitativeResults}, we show some qualitative results of our model trained on synthetic data and tested on synthetic data For this particular qualitative results, we used synthetic data for both training and testing (different images in train and test) to make sure that some examples of our synthetic dataset is exploited to the synthetic dataset. Furthermore, in Figure~\ref{fig:RQualitiveResults} we show results of a model trained on synthetic data, fine-tuned on real data (DCE-1) and tested on real data (DCE-2). By comparing these two figures, we can argue that our model has the potential to be trained on freely made synthetic data and work on real data.



% \begin{figure*}
%     \centering
%     \includegraphics[width=0.7\linewidth]{figures/Supp_DCE_SD_val.pdf}
%     \caption{Qualitative Results of our proposed approach trained on synthetic dataset (5000 images) and tested on a different set of synthetic photos (1000 images).}
%     \label{fig:SDQualitativeResults}
% \end{figure*}

% \begin{figure*}
%     \centering
%     \includegraphics[width=0.7\linewidth]{figures/Supp_DCE_Best_Output.pdf}
%     \caption{Qualitative results of our model trained on synthetic photos (DCE-S) and also fine-tuned on DCE-1, and tested on DCE-2 dataset.}
%     \label{fig:RQualitiveResults}
% \end{figure*}

% % \newpage
% % References should be produced using the bibtex program from suitable
% % BiBTeX files (here: strings, refs, manuals). The IEEEbib.bst bibliography
% % style file from IEEE produces unsorted bibliography list.
% % -------------------------------------------------------------------------
% \bibliographystyle{IEEEbib}
% \bibliography{strings}

% \end{document}
